# Supplementary material for: Evidence for unconventional superconductivity in a spinel oxide
Source: arXiv:2110.13397 source file (2022-08-02)
Supplement: Supplementary file 1 [file LTO_PRX_SM_v2.pdf]

Supplementary Material for

# Evidence for unconventional superconductivity in a spinel oxide

Huanyi Xue[1,*], Lijie Wang[1,*], Zhongjie Wang[1,*], Guanqun Zhang[1], Wei Peng[2,3], Shiwei Wu[1,4], Chunlei Gao[1,4,†], Zhenghua An[1,4,†], Yan Chen[1], and Wei Li[1,†]

[1]State Key Laboratory of Surface Physics and Department of Physics, Fudan University, Shanghai 200433, China

[2]State Key Laboratory of Functional Materials for Informatics, Shanghai Institute of Microsystem and Information Technology, and Center for Excellence in Superconducting Electronics, Chinese Academy of Sciences, Shanghai 200050, China

[3]Center of Materials Science and Optoelectronics Engineering, University of Chinese Academy of Sciences, Beijing 100049, China

[4]Institute for Nanoelectronic Devices and Quantum Computing, Fudan University, Shanghai 200433, China

[*]These authors contributed equally to this work

[†]Correspondence and requests for materials should be addressed to Chunlei Gao (Email: clgao@fudan.edu.cn), Zhenghua An (Email: anzhenghua@fudan.edu.cn), or Wei Li (Email: w_li@fudan.edu.cn).

**This PDF file includes:**

Supplementary text: Sec. I to Sec. VIII
Figs. S1 to S15
Table S1
SM References

## Supplementary Text

**Sec. I. The large-area surface morphology of $MgAl_2O_4$ (001) substrates and $LiTi_2O_4$ (001) thin films.** The atomic force microscopy (AFM) (Asylum Research MFP-3D Classic) is used to observe the surface morphology of $MgAl_2O_4$ (001) substrates and $LiTi_2O_4$ (001) thin films. The large-area surface morphology of $MgAl_2O_4$ (001) substrates after annealing at 800 °C in air for 2 hours and $LiTi_2O_4$ (001) thin films epitaxially grown on $MgAl_2O_4$ are examined by AFM images, shown in Fig. S1(a) and (b), respectively. These results indicate that the low lattice mismatch between $LiTi_2O_4$ and $MgAl_2O_4$ gives rise to the relatively flat surface of films, suggesting high-quality epitaxial growth of $LiTi_2O_4$ thin films on $MgAl_2O_4$.

**Sec. II. The Werthamer-Helfand-Hohenberg (WHH) model fitting.** The WHH model is utilized to quantitatively deduce the effects of the orbital pairing breaking, spin-paramagnetic pair-breaking, and the spin-orbit interaction on the upper critical field shown in Fig. 2(d) and Fig. S3(b). In the dirty limit, the upper critical field can be fitted using the function[22]

$$\ln\frac{1}{t}=\sum_{\nu=-\infty}^{+\infty}\left\{\frac{1}{|2\nu+1|}-\left[|2\nu+1|+\frac{\bar{h}}{t}+\frac{\left(\tilde{\alpha}\bar{h}/t\right)^2}{|2\nu+1|+\left(\bar{h}+\lambda_{so}\right)/t}\right]^{-1}\right\},$$

where $t=T/T_c$, $\bar{h}=\frac{4H_{c2}}{\pi^2H'T_c}$, and $\tilde{\alpha}$ and $\lambda_{so}$ are the parameters reflecting the strength of the spin paramagnetic effect and the spin-orbit interaction, respectively. The $H'$ is a slop at the $T_c$, $H'=-\frac{d\mu_0H_{c2}}{dT}|_{T_c}$, and $\tilde{\alpha}$ is denoted as the Maki parameter. Through the numerical fitting, we evaluate the Maki parameter $\tilde{\alpha}=1.167$ and $\lambda_{so}=50$ for Sample #1 shown in Fig. S3(b), and $\tilde{\alpha}=11.5$ and $\lambda_{so}=35$ for Sample #2 shown in Fig. 2(d). Remarkably, the fitted significantly large strength of spin-orbit interaction $\lambda_{so}$ in the upper critical field implies that the spin-orbit interaction plays a vital role in the electronic conductions in the normal state in $LiTi_2O_4$, which is responsible for the emergence of anomalous magnetoresistance observed in $LiTi_2O_4$[17] (also see Sec. III in details).

**Sec. III. The magnetoresistance and Hall effect measurements in the normal state of $LiTi_2O_4$.** We perform the longitudinal magnetoresistivity $\Delta\rho_{xx} = \rho_{xx}(\mu_0\text{H}) - \rho_{xx}(0\text{ T})$ with an applied out-of-plane magnetic field $\mu_0$H in the normal state in the Sample #1, as shown in Fig. S4(a). The negative magnetoresistivity is found at 80 K. When lowering the temperature, such as the temperature of 25 K, the negative magnetoresistance is disappeared, instead by the positive magnetoresistivity. This anomalous result implies the existence of strong spin fluctuations/spin-orbit coupling effects in the electronic conductions in the normal state in $LiTi_2O_4$, which is consistent with the previous electrical transport measurement[17]. Furthermore, the transverse Hall resistivity $\rho_{xy}$ is also measured on the same footing, as shown in Fig. S4(b). The hole-like charge carrier concentration is thus evaluated to be about $1.8\times10^{22}$ $\text{cm}^{-3}$. In addition, the mobility and the mean free path, as well as the electronic diffusion constant are thus deduced to be $\mu$ = 0.23 $\text{cm}^2/\text{V}\cdot\text{s}$, $l$ = 1.21 nm, and $D_h = 4.87 \times 10^{-3}$ $\text{cm}^2/\text{s}$ at a temperature of 25 K, respectively. These results are in good agreement with previous experiment[17].

**Sec. IV. The first-principles calculations on $LiTi_2O_4$.** The bulk electronic band structure calculations on $LiTi_2O_4$ are performed using the all-electron full potential linear augmented plane wave plus local orbitals (FP-LAPW+lo) method[S1] as implemented in the WIEN2k code[S2]. The exchange-correlation potential is calculated using the generalized gradient approximation as proposed by Perdew, Burke, and Ernzerhof[S3]. Furthermore, a 1000 **k**-point is chosen to ensure the calculations with an accuracy of $10^{-5}$ eV, and all structures (the lattice constants and the internal coordinates) are performed using the values of experimental crystal structure shown in Fig. 1.

Figures S7 and S8 display the electronic band structure for bulk $LiTi_2O_4$ within the framework of density functional theory. Although the spin-orbit coupling (SOC) included in the self-consistent calculations has a lower total energy of 19.4 meV per unit cell than that without inclusion of SOC, the low energy band around the Fermi energy almost remains the same features. Since the SOC breaks the inversion symmetry, the degeneracy at some high symmetric **k**-points is lifted in the inclusion of SOC [Fig. S7(a) and (f)]. In addition, the calculated density of state (DOS) on the non-magnetic (NM) state of $LiTi_2O_4$ is also shown in Fig. S7(b) and (g). We find that the conducting charge carriers

around the Fermi level mainly come from the contributions of Ti 3$d$ orbitals partially hybridized with O 2$p$ orbitals, forming the typical three-dimensional electronic band structured behaviors, which can be seen clearly in the Fermi surface topologies shown in Fig. S7 and the out-of-plane angular-dependent magnetoresistivity (see Fig. S11). Notably, there is a Lifshitz transition point occurring below the Fermi level of 0.1 eV accompanied by the modification of the Fermi surface topologies[S4,S5]. Since the lithium cations are located at the tetrahedral sites, and the titanium cations are occupied the octahedral sites in the spinel structure of $LiTi_2O_4$, we verify the orbital-resolved energy bands and the project DOS on Ti 3$d$ orbitals, and find that the Ti $3d_{x^2-y^2}$ and $3d_{xy}$ orbitals significantly contribute to the electronic conductions around the Fermi level (Fig. S8). On the other hand, the uniformity of electrical conductivity on $LiTi_2O_4$ thin films is also examined experimentally by using the scanning microwave impedance microscopy, which is discussed in details in the subsequent section (see Sec. V in details).

**Sec. V. The uniformity of electrical conductivity on $LiTi_2O_4$ thin films.** To clarify the local uniformity of electrical conductivity on $LiTi_2O_4$ thin films, we systemically carry out the measurements of scanning microwave impedance microscopy (sMIM, LT-ScanWave by PrimeNano), which allows the low temperature conductivity and permittivity measurements ranging from 4 K to 300 K across the superconducting transition temperature of 13 K. The probes with co-axially shielded cantilevers (PrimeNano Inc.) are used to deliver a small microwave excitation with a fixed frequency of 3 GHz. This frequency supports high sensitivity detection of conductivity and permittivity in experiments. The reflected microwave signal is received and analyzed to extract the demodulated output channels: sMIM-R and sMIM-C, which directly indicate the local conductivity and permittivity of the samples, respectively. All the sMIM measurements are conducted in contact mode. In Figs. S9 and S10, the local conductivity and permittivity on the $LiTi_2O_4$ thin films display high uniformity even at elevated temperatures. These results suggest the high uniformity of electrical conductivity on $LiTi_2O_4$ thin films down to the sensitivity limit of the sMIM measurement system.

**Sec. VI. The group symmetry study on the pairing symmetry of $LiTi_2O_4$ superconductor.** In this section, we are going to theoretically discuss the possible symmetry structure of Cooper pairing order parameters of superconducting $LiTi_2O_4$ thin films using the underlying symmetries of the crystal structure without requiring the details of the pairing mechanisms based on the group theoretical formulation of the Ginzburg-Landau theory[S6,S7], which allows us to deduce the fundamental information about the superconducting ground state in $LiTi_2O_4$. Considering the site symmetry of $O_h$ point group in the three-dimensional $LiTi_2O_4$, the superconducting state in $LiTi_2O_4$ is described by the basis function of different irreducible representations of the point group $O_h$ (see Table S1). Here it should be noted that the spatial symmetry group of a solid system is a combination of the point symmetry elements and translations. The latter can be ignored because that the superconducting transition does not bring about an additional spatial modulation. With the help of symmetry group[S6-S10], the possible superconducting order parameters correspond to different irreducible representations of the direct product group, $O_h \times SO(3)$, in the weak spin-orbit coupling limit[S7,S8], where $\times$ and $SO(3)$ represent the direct product and all spin rotations, respectively. Table S1 lists the character table of $O_h$ point group. Therefore, the superconducting pairing gap function is described as

$$\Delta(k) = i\left[\Delta_0(\vec{k})\hat{I} + \vec{d}(\vec{k}) \cdot \hat{\sigma}\right]\sigma_y$$

with $\Delta_0$ corresponding to the one-dimensional singlet representation and the spin vector $\vec{d}$ corresponding to the three-dimensional triplet representation. Here $\hat{\sigma}$ are the Pauli matrices, and $\hat{I}$ is a unit matrix of order 2.

From the group symmetries in the direct product representations[S7,S8] and considering the fact that of experimentally observed fourfold rotational symmetry of superconductivity shown in Fig. 4 and Fig. S11, we inspect the character table of $O_h$ point group listed in Table S1 and notice that only the degenerate basis functions of $d_{x^2-y^2}$-wave and $d_{z^2}$-wave belonging to the two-dimensional irreducible representation of $E_g$ could coincide with the fourfold rotational symmetric structure of angular-dependent $H_{c2}$. Further taking into consideration of the STS measurements shown in Fig. 4(d) (also see Sec. VIII), we demonstrate the superconducting pairing symmetry in the cubic $LiTi_2O_4$ to

be an unconventional $d$-wave with the irreducible representation of $E_g$ protected by $O_h$ point group.

**Sec. VII. Theoretical calculations on the angular-resolved Hall resistivity to further support the *d*-wave pairing in $LiTi_2O_4$ superconductor.** Since the in-plane Hall resistivity $\rho_{xy}$ displays an intriguing opposite sign after the in-plane fourfold rotational operation on rotating the magnetic field direction in the superconducting state shown in Fig. S5(c), we carry out the theoretical calculations to further quantitatively support the intrinsic in-plane $d$-wave Cooper pairing formation of superconducting $LiTi_2O_4$. Theoretically, the in-plane transverse Hall resistivity can be written as $\rho_{xy} = -\rho_{yx} = -\frac{\sigma_{xy}}{\sigma_{xx}^2+\sigma_{xy}^2}$, where $\sigma_{xx}$ and $\sigma_{xy}$ are longitudinal and transverse Hall conductivity, respectively. When a small electric field is applied, a resulting current is given by the response (Kubo) formula[S11]. A linear response of current in the perpendicular direction to the applied electric field is represented by the Hall conductance[S12],

$$\sigma_{xy} = -ie^2\hbar \sum_{E^\alpha<E_f<E^\beta} \frac{(v_y)_{\alpha\beta}(v_x)_{\beta\alpha} - (v_x)_{\alpha\beta}(v_y)_{\beta\alpha}}{(E^\alpha - E^\beta)^2}$$

where $E_f$ is a Fermi energy and the summation implies the sum over all the states below and above the Fermi energy. The indices $\alpha$ and $\beta$ label the electronic bands. Importantly, the Hall conductance can be simplified as a relation to the Berry phase[S13],

$$\sigma_{xy}^\alpha = \frac{e^2}{h}\frac{1}{2\pi i}\int d^2k\hat{k}_z \cdot [\nabla_k \times \boldsymbol{\mathcal{A}}_\alpha(\vec{k})] = \frac{e^2}{h}\frac{1}{2\pi i}\int_C d\vec{k} \cdot \boldsymbol{\mathcal{A}}_\alpha(\vec{k})$$

Here $\boldsymbol{\mathcal{A}}_\alpha(\vec{k}) = \langle\Psi_\alpha|\nabla_{\vec{k}}|\Psi_\alpha\rangle$ is the Berry connection, and $|\Psi_\alpha\rangle$ is the eigenstate corresponding to the eigenenergy $E_\alpha$. Thus, the experimentally observed in-plane angle $\varphi$-dependent transverse Hall resistivity $\rho_{xy}(\varphi)$ is proportional to the structural formation of Berry connection in the Brillouin zone.

Next, we perform the theoretical calculations on a simplified two-dimensional anisotropic $d_{x^2-y^2}$-wave superconductivity, which could provide a significant insight into the nontrivial topological properties of the superconducting Cooper pairs linked to the rotational symmetric structure of in-plane angular-dependent $\rho_{xy}(\varphi)$ shown in Fig. S5(c).

The simplified theoretical model is written by the Bogoliubov-de Gennes (BdG) Hamiltonian,

$$\hat{H} = \begin{pmatrix} H_0(\vec{k}) & \Delta_0(\vec{k}) \\ \Delta_0^\dagger(\vec{k}) & -H_0(-\vec{k}) \end{pmatrix}$$

where $\vec{k}$ is the momentum of the excitation, $H_0(\vec{k}) = -2t_0(\cos k_x + \cos k_y) - \mu$ describes a normal free electron Hamiltonian, and $\Delta_0(\vec{k}) = \Delta_0(\cos k_x - \cos k_y)$ represents the superconducting pairing potential. Throughout the theoretical calculations, we set $t_0$ as an energy unit and $\mu = 0$. The energy dispersion as functions of $k_x$ and $k_y$ is diagonalized and shown in Fig. S13(a). Importantly, it is worth pointing out that there are four nodes located at the Fermi surface. The Berry connection is easily evaluated under its definition[S11], $\boldsymbol{\mathcal{A}}_n(\vec{k}) = \langle \Psi_n | \nabla_{\vec{k}} | \Psi_n \rangle$ , shown in Fig. S13(b), and displays the singularities at the nodes of the Fermi surface. By projecting the Berry connection vector $\boldsymbol{\mathcal{A}}_n(\vec{k})$ onto the direction of in-plane angle $\varphi$, we find $\boldsymbol{\mathcal{A}}_{\boldsymbol{\varphi}}$ to be oscillated periodically and the singularities are located at the in-plane angles of $\varphi = \frac{\pi}{4}, \frac{3\pi}{4}, \frac{5\pi}{4}$, and $\frac{7\pi}{4}$ [see Fig. S13(c)], consistent with the Berry connection calculations. These results imply the existence of non-trivial topological properties at the nodes. The topological nontrivial winding number is thus evaluated to $N_w = \pm 1$ at the nodes[S14,S15], as shown in Fig. S13(a) and (b). These non-zero values of winding number are protected by the time-reversal symmetry, since the total winding over the Brillouin zone must be zero in an anisotropic $d_{x^2-y^2}$-wave superconductor. Furthermore, the non-zero winding number will be responsible for the appearance of anomalous Hall-like conductance when the current flows along node directions, $\varphi = \frac{\pi}{4}, \frac{3\pi}{4}, \frac{5\pi}{4}$, and $\frac{7\pi}{4}$, leading to the sign change at the nodes in the transverse Hall resistivity $\rho_{xy}$ due to the sign change in the winding number. On the other hand, according to the bulk-boundary correspondence[S16], the edge states are also carried out for the theoretical calculations. As we expected that Fig. S13(d) shows the appearance of edge states when the edge is along the [1,1]-direction. These calculations are consistent with the experimental observation in the in-plane angular-resolved transverse Hall resistivity $\rho_{xy}$ shown in Fig. S5(c). More importantly, we further demonstrate the correspondence between the rotational symmetric structure of the $\rho_{xy}$ in

the superconducting state and the superconducting Cooper pairs, making it a new experimental probe with phase sensitivity to detect a definite fingerprint of the pairing symmetry of superconducting Cooper pairs.

**Sec. VIII. Scanning tunneling microscopy (STM) topography and STS fitting using the Dynes formula.** In order to gain further information, such as the superconducting gap, on the spinel oxide superconductor, a preliminary STM measurement is carried out in $LiTi_2O_4$ (001) films. Figure S14(a) shows the STM topographic image of the $LiTi_2O_4$ (001) film. One can see from this topography that the surface of $LiTi_2O_4$ film is relatively flat and homogeneous in such large area [Fig. S14(b) and (c)]. The tunneling spectra are also found to be homogeneous when the measurements go along the black arrowed line with the lengths of about 30 nm [Fig. S14(d)]. The uniformity of the superconducting gap spectra indicates that the superconductivity of $LiTi_2O_4$ films are homogeneous with high quality. All the spectra consistently display a pronounced V-shaped-like feature [also see Fig. 4(d)], which points to a common origin of the *d*-wave superconducting pairing.

To quantitatively evaluate the superconducting gap $\Delta_g$, we fit the tunneling spectra using the Dynes formula[33,34]:

$$\frac{dI}{dV}(eV_s,T) = -a\int_{-\infty}^{+\infty}\int_{-\infty}^{+\infty}[\rho(E)f'(\epsilon+E,T)dE]\,b(eV_s-\epsilon)d\epsilon.$$

This equation represents the density of state from sample $\rho(E)$ convolved with the thermal broadening $f'(E,T)$ and bias modulation broadening $b(V_s)$[34], where $e$ and $V_s$ are the elementary charge and the bias voltage, respectively. Here, we adopt Dynes function with the spectral broadening factor $\Gamma$ for the sample[33],

$$\rho_D(E) = \mathrm{Re}\left(\frac{E-i\Gamma}{\sqrt{(E-i\Gamma)^2-\Delta_g^2}}\right)$$

The $f'(E,T)$ is the derivative of Fermi function and $b(V_s)$ is the known lock-in broadening function,

$$f'(\epsilon,T) = \frac{df(\epsilon,T)}{d\epsilon} = -\frac{\exp(\epsilon/k_BT)}{k_BT[\exp(\epsilon/k_BT)+1]^2}$$

$$b(V_s) = \begin{cases} \frac{\sqrt{2}}{\pi V_{mod}} \sqrt{1 - \left(\frac{V_s}{\sqrt{2} V_{mod}}\right)^2}, & (|V_s| \leq \sqrt{2} V_{mod}) \\ 0, & (|V_s| > \sqrt{2} V_{mod}) \end{cases}$$

where $V_{mod}$ is the root-mean-square amplitude of lock-in excitation. The fitting parameters $a$, $\Delta_g$, and Γ are determined with the fixed temperature of $T$ = 4.2 K. We fit our spectra [Fig. 4(d)] with a single-component isotropic *s*-wave pairing gap and an anisotropic *d*-wave pairing gap with the two-dimensional irreducible representation of $E_g$ [$d_{x^2-y^2}+d_{z^2}$-wave with the gap function of $\Delta_g \left(\frac{\sqrt{3}}{2} \sin^2\theta \cos 2\phi + \frac{1}{2}(3\cos^2\theta - 1)\right)$, here $\theta$ and $\phi$ are the out-of-plane polar and in-plane azimuthal angles, respectively][S6,S7] (see the detailed discussions on Sec. VI), and thus obtain the $\Delta_g = 2.21$ meV and $\Gamma = 0.01$ meV for the isotropic *s*-wave pairing state and $\Delta_g = 2.4$ meV and $\Gamma = 0.01$ meV for the *d*-wave pairing state. Obviously, only the anisotropic *d*-wave pairing state can well reproduce the fundamental feature of V-shaped-like tunneling conductance in STS in $LiTi_2O_4$.

On the other hand, by tuning the various values of spectral broadening parameter Γ and the *s*-wave gap amplitude $\Delta_g$ shown in Fig. S15, we find that none of them could reproduce the main feature of the tunneling conductance in STS, suggesting that the extrinsic spectral broadening in the *s*-wave pairing state is unlikely to the source of our experimentally observed V-shaped-like feature in the tunneling conductance in STS, and thus, we attribute this V-shaped-like feature in the tunneling conductance in STS to the intrinsic nature of *d*-wave superconducting pairing state in $LiTi_2O_4$.

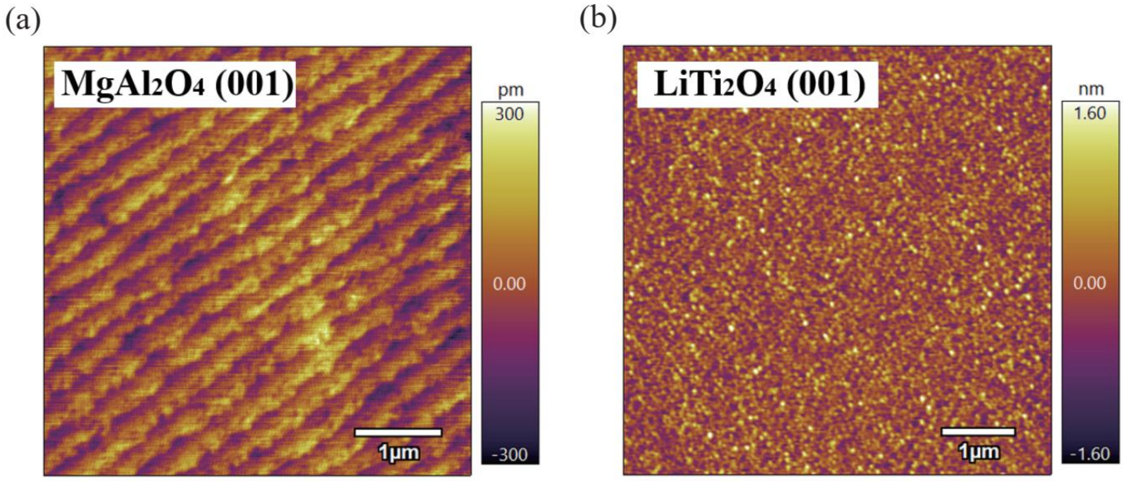


**Fig. S1.** Large-area AFM images of (a) $MgAl_2O_4$ (001) substrate and (b) $LiTi_2O_4$ (001) thin film.

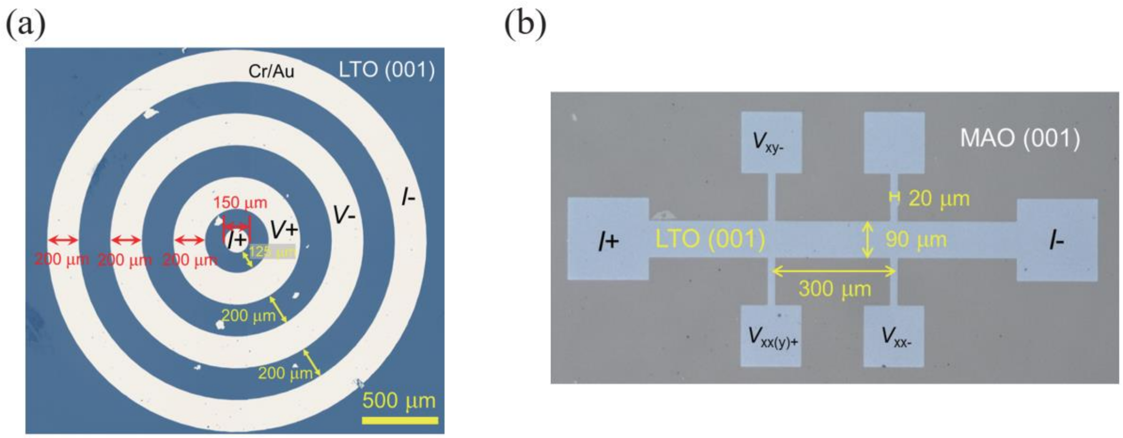


**Fig. S2.** Optical microscopic images of the fabricated structure of $LiTi_2O_4$ (LTO) (001) thin films grown on the $MgAl_2O_4$ (MAO) (001) substrates with (a) Corbino and (b) Hall bar devices. The precise geometries of the devices are documented in the figures. Here, the Corbino disk is fabricated by depositing 8 nm thick Cr and 100 nm thick Au layers on a patterned LTO surface, and the Hall bar structure is fabricated by UV photolithography and argon ion etching.

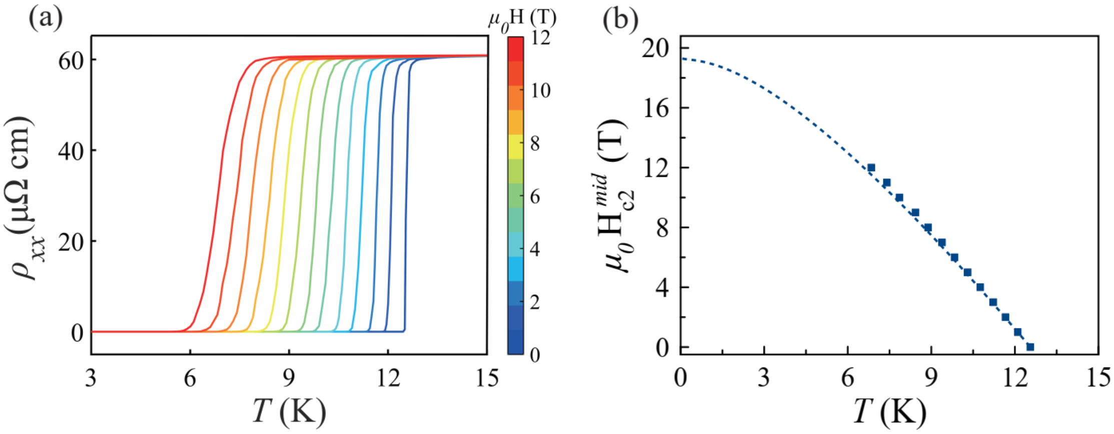


**Fig. S3.** Superconducting properties of $LiTi_2O_4$ (001) thin film. (a) Magnetoresistivity for fields perpendicular to the plane surface of Sample #1. (b) Temperature-dependent upper critical fields $\mu_0 H_{c2}^{mid}$, which are determined at half the values of $\rho_{xx}$ in (a). The blue dashed line is fitted by WHH theory.

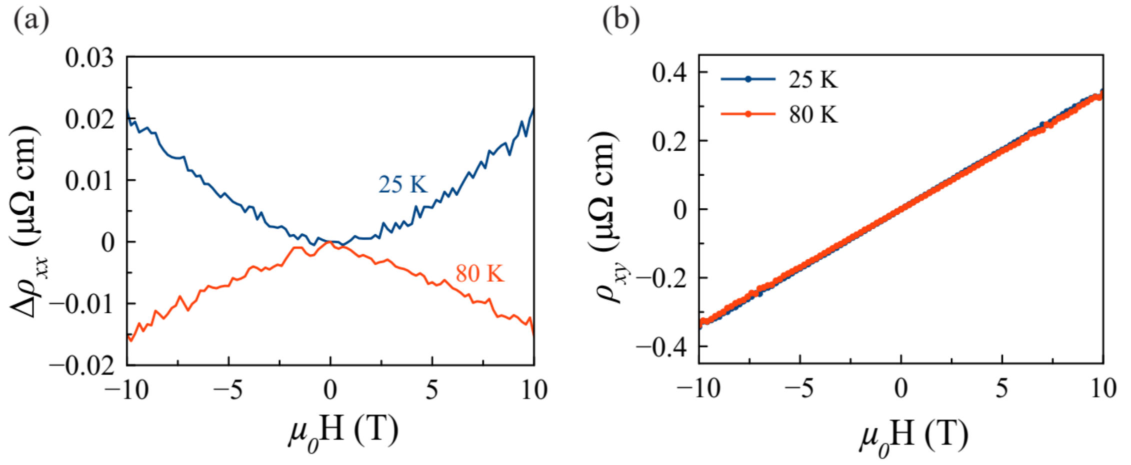


**Fig. S4.** (a) Longitudinal magnetoresistivity with an applied out-of-plane magnetic field $\mu_0$H, $\Delta\rho_{xx} = \rho_{xx}(\mu_0\mathrm{H}) - \rho_{xx}(0\ \mathrm{T})$, with fixed temperatures of 25 and 80 K on Sample #1. The $\Delta\rho_{xx}$ changes from positive to negative for the temperatures of 25 and 80 K, implying the existence of strong spin fluctuations/spin-orbit coupling in the electronic conductions in the normal state in $LiTi_2O_4$[17]. (b) Corresponding transverse Hall resistivity $\rho_{xy}$. The hole-like charge carrier concentration is evaluated to be $1.8\times10^{22}$ $cm^{-3}$, which is in good agreement with previous experiment[17].

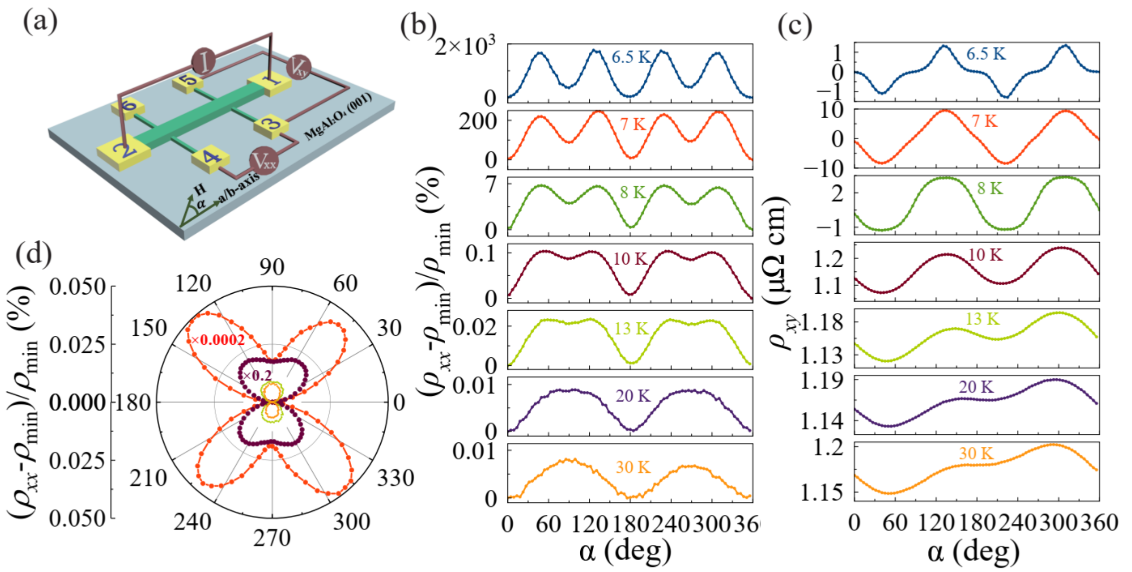


**Fig. S5.** Temperature-dependent electrical resistivity on the Hall bar structure of $LiTi_2O_4$ (001) thin film. (a) Schematic image of the Hall bar device for in-plane angular-dependent longitudinal magnetoresistivity ($\rho_{xx}$) and transverse Hall resistivity ($\rho_{xy}$) measurements. (b) Temperature-dependent longitudinal magnetoresistivity $\rho_{xx}$ normalized by minimum value of $\rho_{xx}$ ($\rho_{min}$) with the fixed field of $\mu_0$H = 12 T. (c) Temperature-dependent transverse Hall resistivity $\rho_{xy}$ with fixed the same field of $\mu_0$H = 12 T. (d) Corresponding polar plot of the temperatures of 7 K, 10 K, 13 K, and 30 K in (b). Here, it should be noted that the existence of in-plane twofold rotational symmetry in the longitudinal magnetoresistivity $\rho_{xx}$ in the normal state in the Hall bar structure mainly originates from the extrinsic contribution of Lorentz force as evidenced by the minimum of $\rho_{xx}$ for a field parallel to the current and maximum of $\rho_{xx}$ for a field perpendicular to the current. In the superconducting state, we find the emergence of fourfold rotational symmetry in magnetoresistivity $\rho_{xx}$, suggestive of the unconventional superconductivity in $LiTi_2O_4$ owing to the *d*-wave pairing state. Furthermore, the amplitude of transverse Hall resistivity $\rho_{xy}$ also exhibits fourfold rotational symmetry, and the phases of $\rho_{xy}$ change their sign oppositely after the in-plane fourfold rotational operation on rotating magnetic field direction in the superconducting state in (c), excluding a possible *s*-wave state with small gap minima and providing a compelling indication for the intrinsic in-plane *d*-wave superconducting pair in $LiTi_2O_4$.

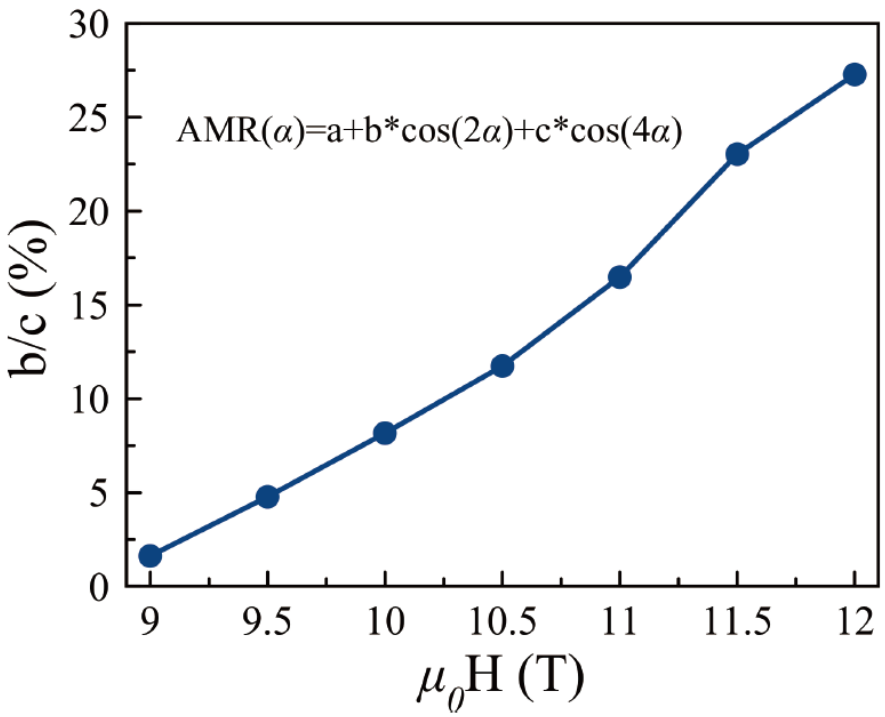


**Fig. S6.** Field-dependent ratio of twofold and fourfold components in $LiTi_2O_4$ (001) thin film. The in-plane azimuthal angle $\alpha$-dependent anisotropic magnetoresistivity [AMR, a+b*cos (2$\alpha$)+c*cos (4$\alpha$), as shown in the inset of figure] is fitted to the data shown in Fig. 3(d). Here, it should be noted that the negligible component of twofold symmetry is immersed in the in-plane azimuthal angular-dependent magnetoresistivity $\rho_{xx}$ [$T$ = 8 K in Fig. 3(b)], and becomes enhanced with increasing field [also see Fig. 3(d)], implying that this twofold symmetry component in magnetoresistivity at the superconducting phase transition region mainly originates from the extrinsic contribution induced by the applied field, such as the magnetic field induced vortex dynamics or a possible effect of the misalignment of the field with the film plane.

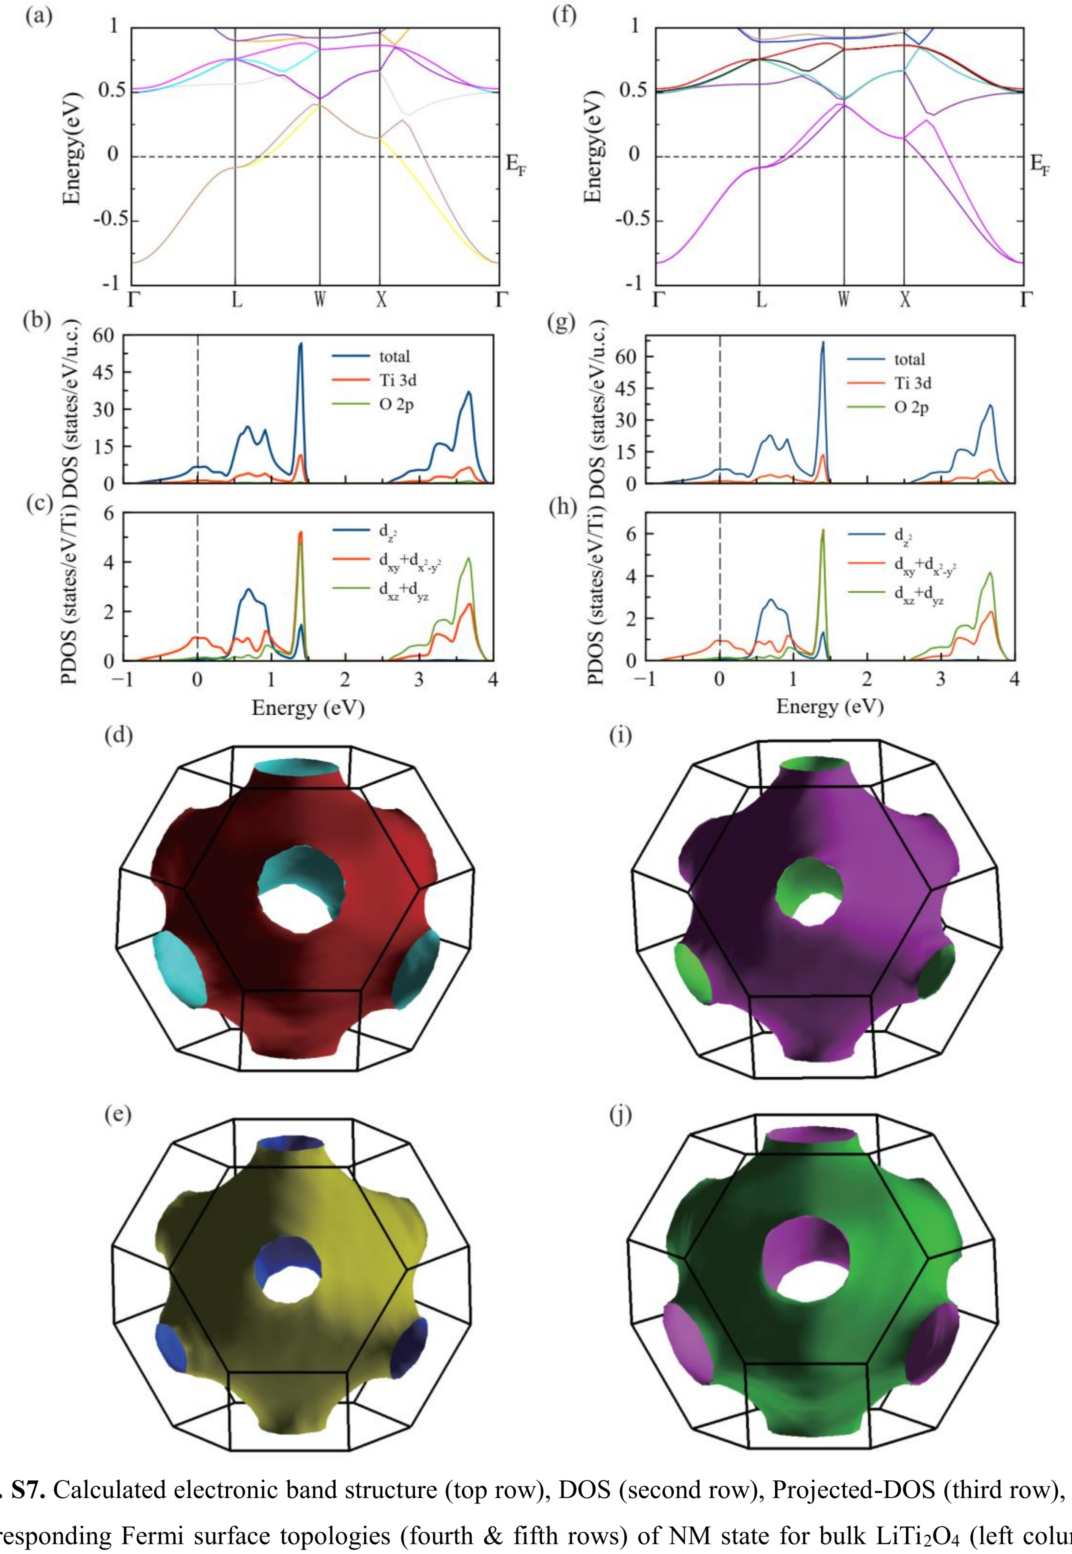


**Fig. S7.** Calculated electronic band structure (top row), DOS (second row), Projected-DOS (third row), and corresponding Fermi surface topologies (fourth & fifth rows) of NM state for bulk $LiTi_2O_4$ (left column) with and (right column) without SOC. The Fermi level is set to zero.

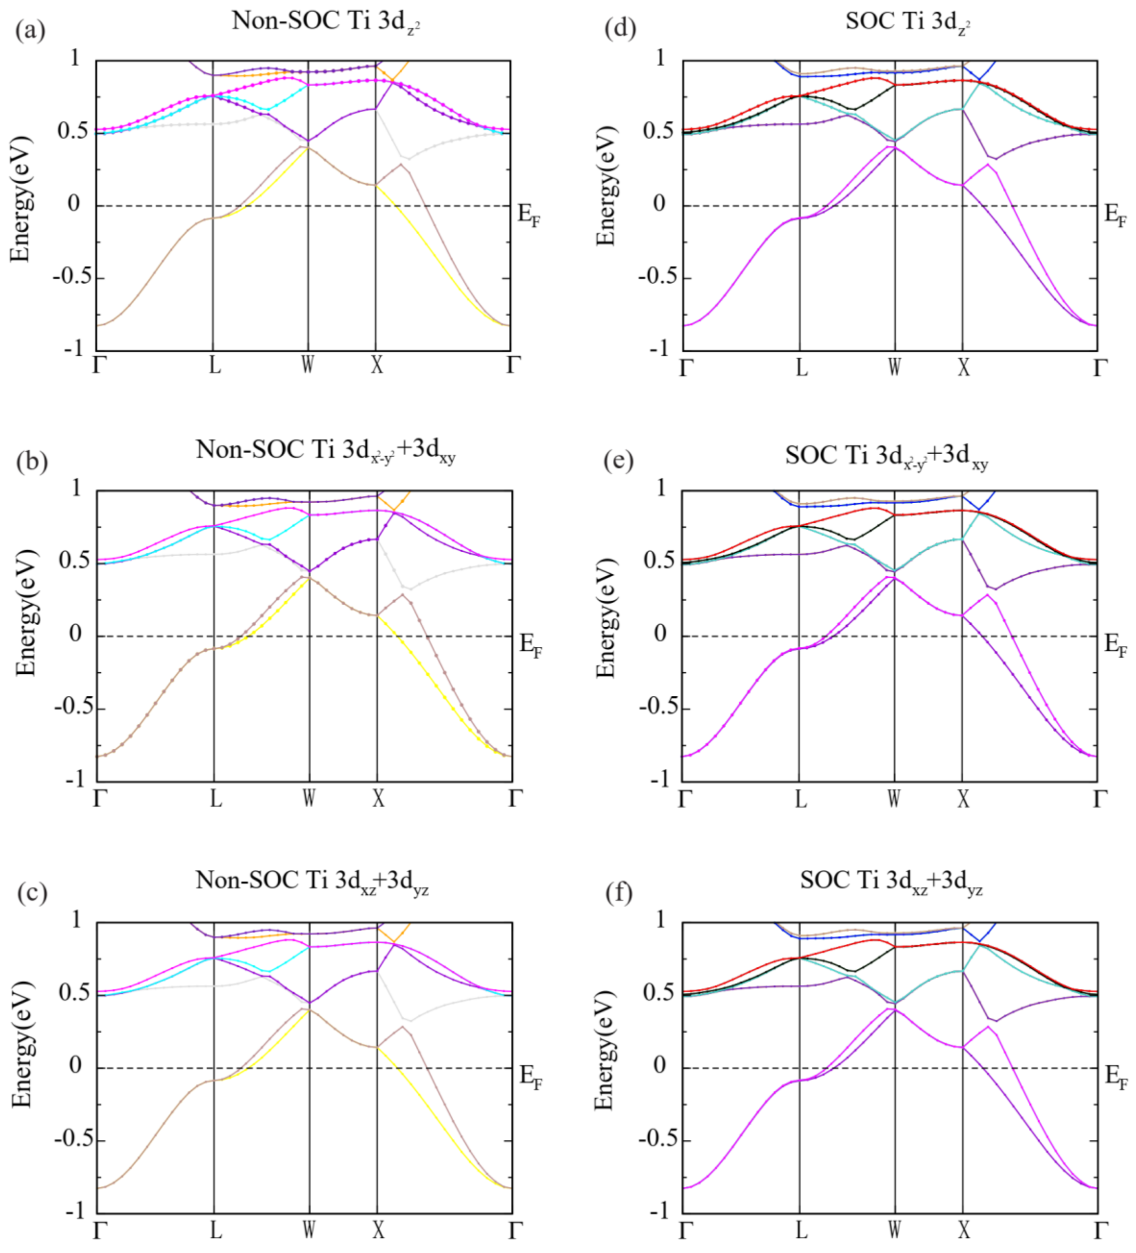


**Fig. S8.** Ti 3*d* orbitals resolved energy bands with NM state for bulk of $LiTi_2O_4$ (left column) with and (right column) without SOC. The Fermi level is set to zero.

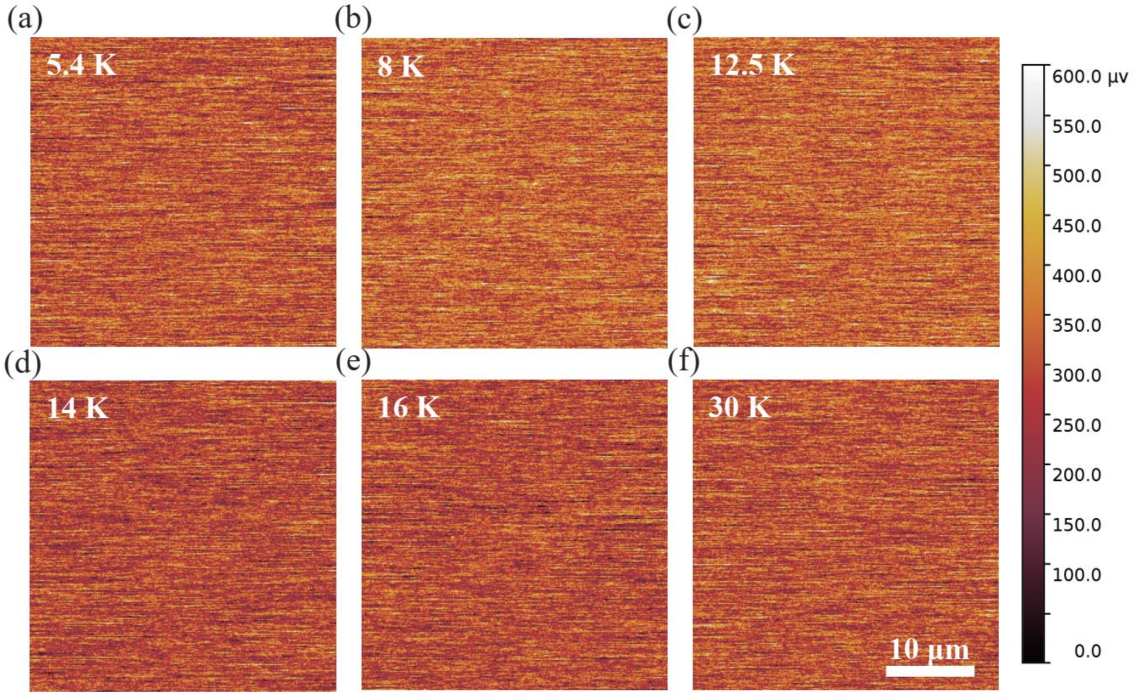


**Fig. S9.** sMIM-R images of $LiTi_2O_4$ (001) thin films under various temperatures. The sMIM-R directly indicates the local high uniformity of conductivity of the sample area.

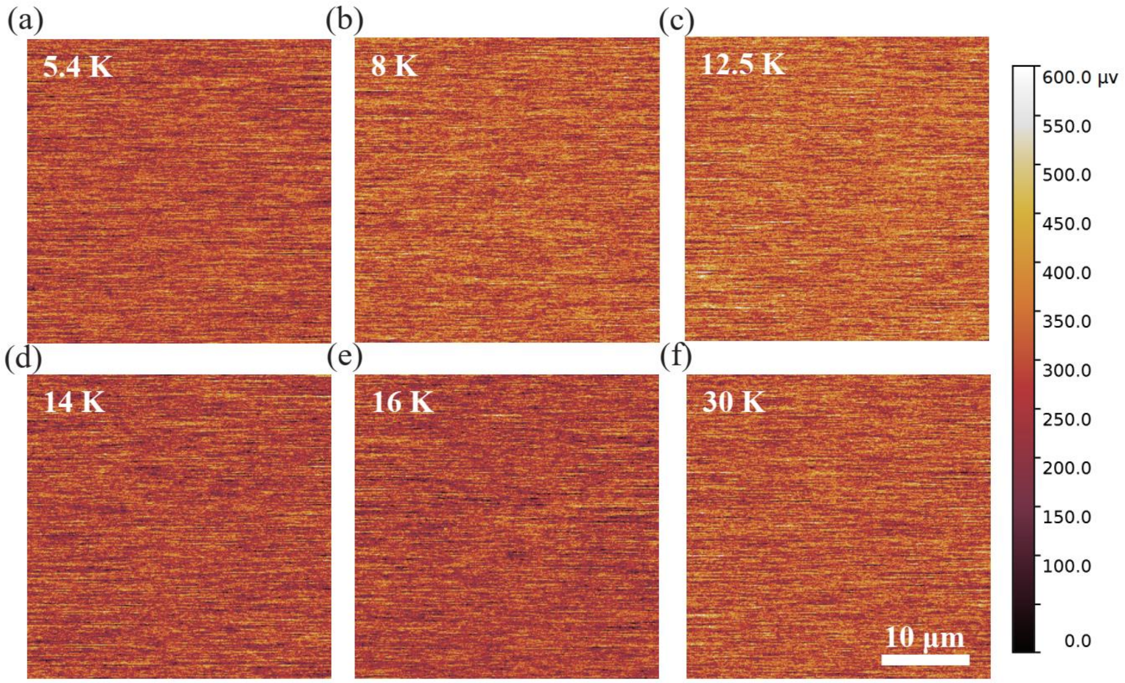


**Fig. S10.** sMIM-C images of $LiTi_2O_4$ (001) thin films under various temperatures. The sMIM-C directly indicates the local high uniformity of permittivity of the sample area.

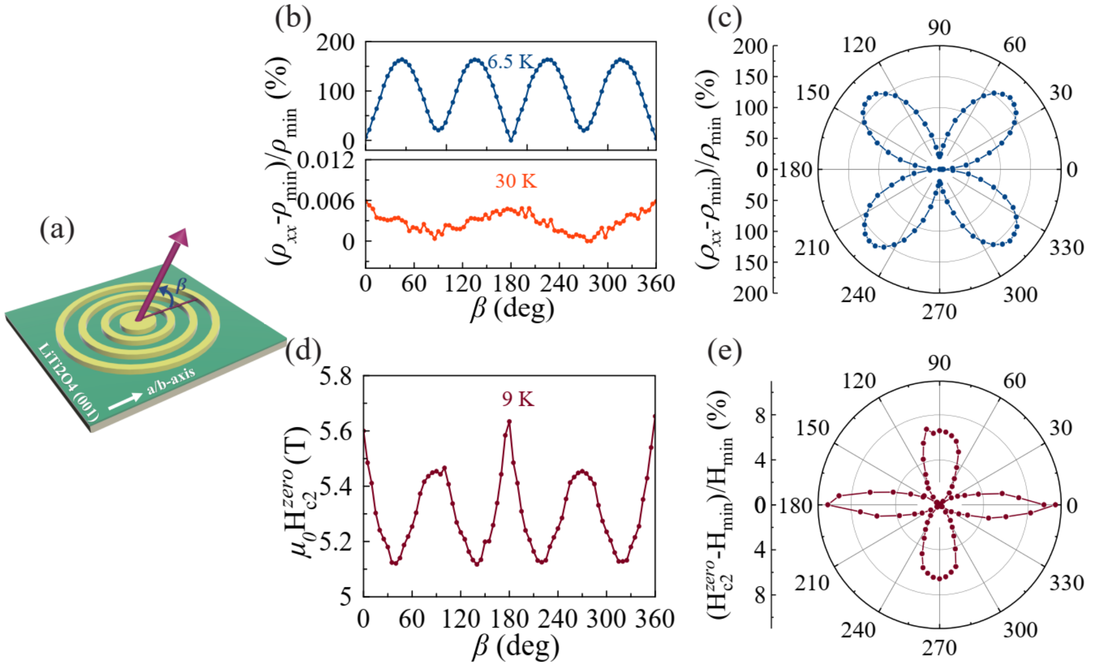


**Fig. S11.** Out-of-plane fourfold modulations in the Corbino structure of $LiTi_2O_4$ (001) thin film. (a) Schematic image of the Corbino-shaped device for the out-of-plane polar angular-dependent magnetoresistivity ($\rho_{xx}$) measurements. The out-of-plane polar angle $\beta$ is set to zero ($\beta = 0$) when the field is applied parallel to $LiTi_2O_4$ plane surface along the a/b-axis. (b) Temperature-dependent $\rho_{xx}$ normalized by minimum value of $\rho_{xx}$ ($\rho_{min}$) with fixed field of $\mu_0$H = 12 T. (c) Corresponding polar plot of the temperature of 6.5 K in (b). (d) Out-of-plane polar angular-dependent $\mu_0 H_{c2}^{zero}$ at 9 K. (e) Polar plots of the data normalized by the minimum value of $H_{c2}^{zero}$ ($H_{min}$) in (d). Here, the out-of-plane fourfold modulations are clearly visible in both the magnetoresistivity $\rho_{xx}$ and upper critical field $\mu_0 H_{c2}^{zero}$ in the superconducting state, providing an additional evidence for the *d*-wave superconducting Cooper pair formation with the irreducible representation of $E_g$ in the three-dimensional spinel oxide $LiTi_2O_4$.

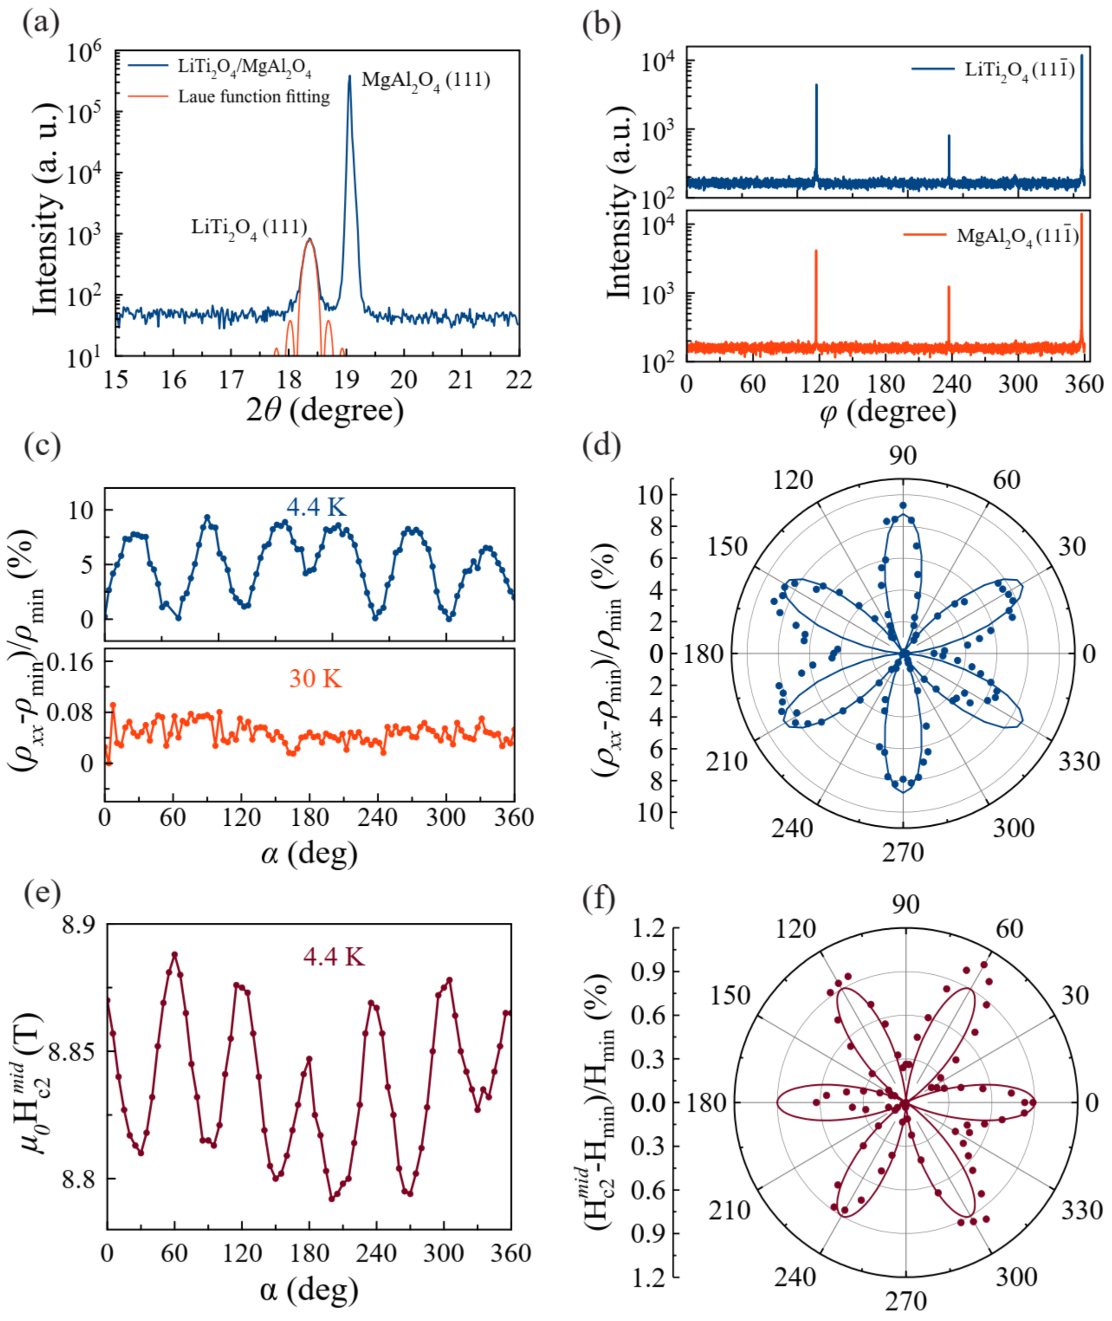


**Fig. S12.** Signature of in-plane sixfold superconducting behavior in $LiTi_2O_4$ (111) thin film. (a) $2\theta$ XRD spectrum of an epitaxial $LiTi_2O_4$ (111) thin film grown on a $MgAl_2O_4$ (111) substrate using the same growth conditions to that of $LiTi_2O_4$ (001) films. The thickness of the $LiTi_2O_4$ (111) thin film is estimated to be 38.6 nm deduced from the formula of Laue oscillation. (b) $\varphi$-scan of the $\{11\bar{1}\}$ diffraction planes for the $LiTi_2O_4$ (111) film and $MgAl_2O_4$ (111) substrate. Three peaks are uniformly distributed, displaying the in-plane threefold rotational symmetry of the lattice and implying in-plane epitaxy. (c) Temperature-dependent longitudinal magnetoresistivity $\rho_{xx}$ normalized by minimum value of $\rho_{xx}$ ($\rho_{min}$) with the fixed field of $\mu_0 H$ = 9 T on the Hall bar structure. (d) Corresponding polar plot of the temperature of 4.4 K in (c). (e) In-plane

angular-dependent $\mu_0 H_{c2}^{mid}$ at temperature of 4.4 K. Here, $H_{c2}^{mid}$ is extracted at the midpoints of magnetoresistivity $\rho_{xx}$. (f) Polar plots of the data normalized by the minimum value of $H_{c2}^{mid}$ ($H_{min}$) in (e). Here, the in-plane sixfold modulations are clearly visible in the magnetoresistivity $\rho_{xx}$ and upper critical field $\mu_0 H_{c2}^{mid}$ in the superconducting state in $LiTi_2O_4$ (111) films, providing an additional evidence for the $d$-wave superconducting Cooper pair formation with the irreducible representation of $E_g$ in three-dimensional spinel oxide $LiTi_2O_4$.

**Table S1.** Character table for point group of $O_h$.

| $O_h$ | E | $8C_3$ | $6C_2$ | $6C_4$ | $3C_2=(C_4)^2$ | i | $6S_4$ | $8S_6$ | $3\sigma_h$ | $6\sigma_d$ | linear functions, rotations | quadratic functions | cubic functions |
|---|---|---|---|---|---|---|---|---|---|---|---|---|---|
| $A_{1g}$ | 1 | +1 | +1 | +1 | +1 | +1 | +1 | +1 | +1 | +1 | - | $x^2+y^2+z^2$ | - |
| $A_{2g}$ | 1 | +1 | -1 | -1 | +1 | +1 | -1 | +1 | +1 | -1 | - | - | - |
| $E_g$ | 2 | -1 | 0 | 0 | +2 | +2 | 0 | -1 | +2 | 0 | - | $(2z^2-x^2-y^2, x^2-y^2)$ | - |
| $T_{1g}$ | 3 | 0 | -1 | +1 | -1 | +3 | +1 | 0 | -1 | -1 | $(R_x, R_y, R_z)$ | - | - |
| $T_{2g}$ | 3 | 0 | +1 | -1 | -1 | +3 | -1 | 0 | -1 | +1 | - | $(xz, yz, xy)$ | - |
| $A_{1u}$ | 1 | +1 | +1 | +1 | +1 | -1 | -1 | -1 | -1 | -1 | - | - | - |
| $A_{2u}$ | 1 | +1 | -1 | -1 | +1 | -1 | +1 | -1 | -1 | +1 | - | - | $xyz$ |
| $E_u$ | 2 | -1 | 0 | 0 | +2 | -2 | 0 | +1 | -2 | 0 | - | - | - |
| $T_{1u}$ | 3 | 0 | -1 | +1 | -1 | -3 | -1 | 0 | +1 | +1 | $(x, y, z)$ | - | $(x^3, y^3, z^3)$ $[x(z^2+y^2), y(z^2+x^2), z(x^2+y^2)]$ |
| $T_{2u}$ | 3 | 0 | +1 | -1 | -1 | -3 | +1 | 0 | +1 | -1 | - | - | $[x(z^2-y^2), y(z^2-x^2), z(x^2-y^2)]$ |

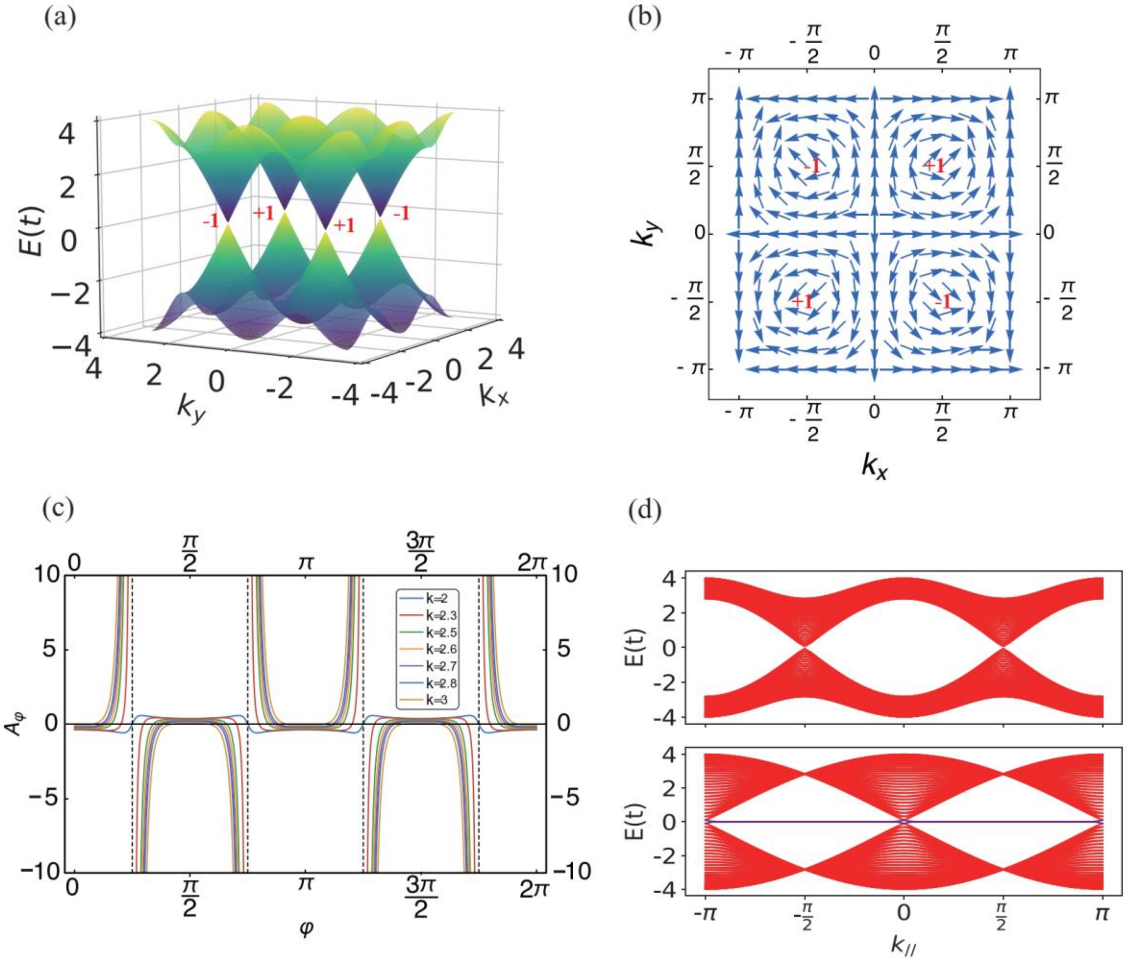


**Fig. S13.** Theoretical calculations on the topological structure of the *d*-wave pairing state. (a) The dispersion of anisotropic layered $d_{x^2-y^2}$-wave superconductor. (b) Corresponding Berry connection $\mathcal{A}_n(\vec{k})$. (c) Projecting the Berry connection vector into the in-plane azimuthal angle ($\varphi$) direction $\mathcal{A}_{\varphi}$. (d) The dispersion for a ribbon along the edge of [0,1] direction (top) and [1,-1] direction (bottom). The evaluated winding numbers are shown in (a) and (b). These theoretical calculations imply that the Hall resistivity $\rho_{xy}$ displays an opposite sign after the in-plane fourfold rotational operation, which is consistent with the Hall measurements shown in Fig. S5(c), and thus demonstrate the intrinsic *d*-wave paring nature of $LiTi_2O_4$ superconductor.

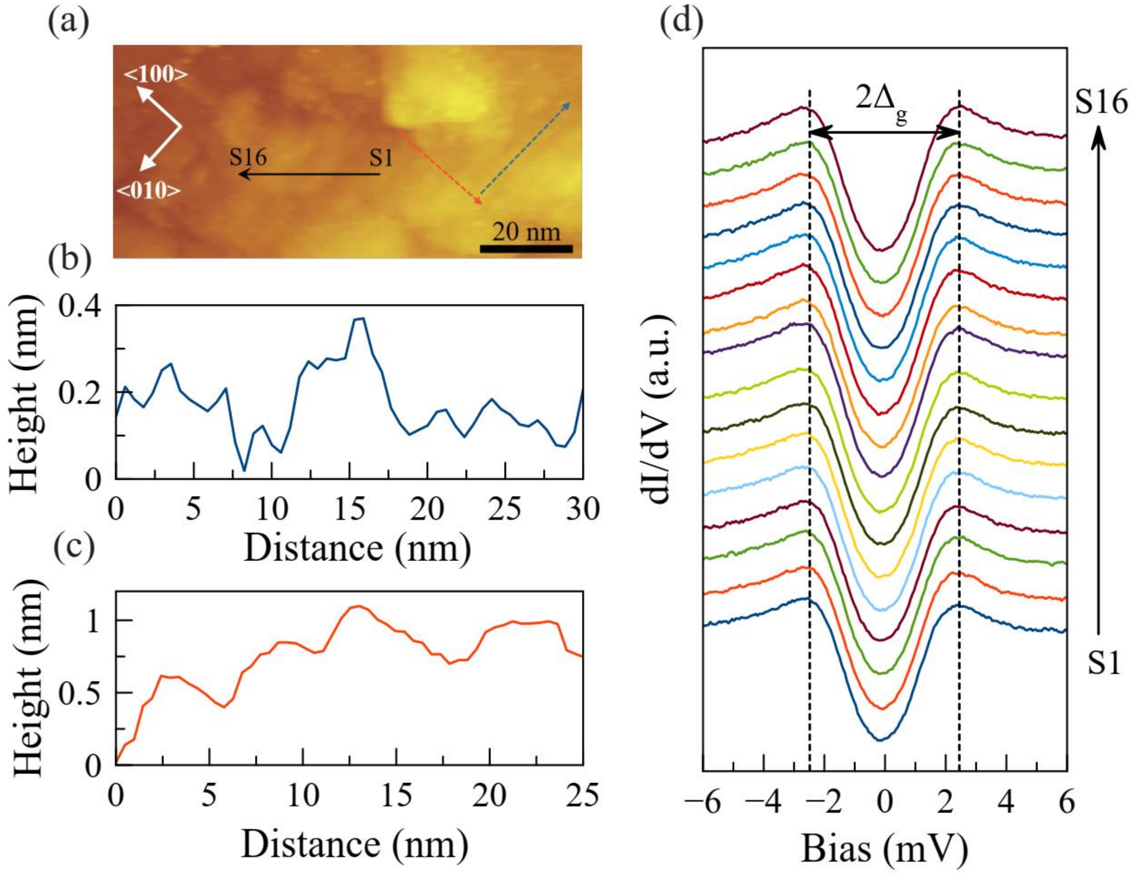


**Fig. S14.** Large-scale STM topography and spatial dependence of *dI/dV* spectra on $LiTi_2O_4$ (001) films. (a) STM topographic image of the $LiTi_2O_4$ (001) surface. (b) and (c) Line profiles along the blue and red arrow dashed lines as indicated in (a). (d) A series of *dI/dV* spectra acquired along the trajectory in (a). The spectra are shifted for clarity and the black dashes indicate the energy positions of the superconducting gap ($2\Delta_g$). Set-point conditions for measuring the spectrum are $V_{set}$ = 6 mV and $I_{set}$ = 100 pA.

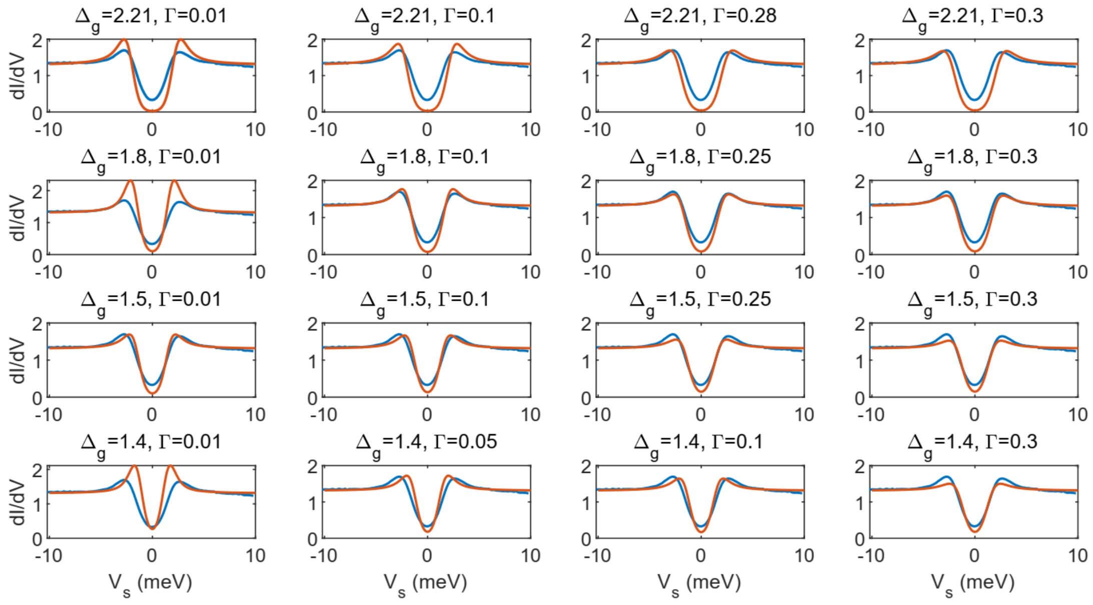


**Fig. S15.** Ruling out the possibility of *s*-wave superconducting pairing in the tunneling conductance in STS using the Dynes formula fitting. Tuning the various values of broadening Γ and the *s*-wave gap amplitude $\Delta_g$ (red solid lines), we find that none of them could reproduce the main feature of the tunneling conductance in STS with fixed temperature of 4.2 K, and thus exclude the *s*-wave pairing state for the nature of the V-shaped-like feature (blue solid line) observed in the tunneling conductance in STS.

**SM References**


S1. D. Singh and L. Nordström, *Planewaves, Pseudopotentials and the LAPW Method*, $2^{nd}$ edm (Springer-Verlag, Berlin, 2005).

S2. P. Blaha, K. Schwarz, G. Madsen, D. Kvasnicka, and J. Luitz, *WIEN2k: An Augmented Plane Wave plus Local Orbitals Program for Calculating Crystal Properties* (Technical Univievsity Wien, Austria, 2001).

S3. J. P. Perdew, K. Burke, and M. Ernzerhof, *Generalized Gradient Approximation Made Simple*, Phys. Rev. Lett. **77**, 3865 (1996).

S4. M. I. Lifshitz, *Anomalies of electron characteristics of a metal in the high pressure region*, Sov. Phys. JETP **11**, 1130 (1960).

S5. G. E. Volovik, *Topological Lifshitz transitions*, Low Temp. Phys. **43**, 47 (2017).

S6. R. Evarestov and V. Smirnov, *Site Symmetry in Crystals* (Springer-Verlag, Berlin, 1997).

S7. M. Sigrist and K. Ueda, *Phenomenological theory of unconventional superconductivity*, Rev. Mod. Phys. **63**, 239 (1991).

S8. J. F. Annett, *Symmetry of the order parameter for high-temperature superconductivity*, Adv. Phys. **39**, 83 (1990).

S9. M. Zou, J. Chu, H. Zhang, T. Yuan, P. Cheng, W. Jin, D. Jiang, X. Xu, W. Yu, Z. An, X. Wei, G. Mu, and W. Li, *Evidence for ferromagnetic order in the CoSb layer of* $LaCoSb_2$, Phys. Rev. B **101**, 155138 (2020).

S10. T.-Z. Yuan, M.-Y. Zou, W.-T. Jin, X.-Y. Wei, X.-G. Xu, and W. Li, *Pairing symmetry in monolayer of orthorhombic CoSb*, Front. Phys. **16**, 43500 (2021).

S11. D. J. Thouless, M. Kohmoto, M. P. Nightingale, and M. den Nijs, *Quantized Hall conductance in a two-dimensional periodic potential*, Phys. Rev. Lett. **49**, 405 (1982).

S12. M. Kohmoto, *Topological invariant and the quantization of the Hall conductance*, Ann. Phys. **160**, 343 (1985).

S13. D. Xiao, M.-C. Chang, and Q. Niu, *Berry phase effects on electronic properties*, Rev. Mod. Phys. **82**, 1959 (2010).

S14. X. G. Wen and Z. Zee, *Gapless fermions and quantum order*, Phys. Rev. B **66**, 235110 (2002).

S15. W. G. Unruh and R. Schützhold, *Quantum analogues: From phase transitions to black holes and cosmology* (Springer, Berlin Heidelberg, 2007).

S16. Y. Hatsugai, *Chern number and edge states in the integer quantum Hall effect*, Phys. Rev. Lett. **71**, 3697 (1993).
